# Supplementary material for: Trackable Agent-based Evolution Models at Wafer Scale
Source: arXiv:2404.10861 source file (2024-06-02)
Supplement: Supplementary file 3 [file supplement.tex]

\section{Supplemental Material}

\section{Example} \label{sec:example}

example \citep{gropp1996high}
